# Supplementary material for: Learning Wheelchair Tennis Navigation from Broadcast Videos with Domain Knowledge Transfer and Diffusion Motion Planning
Source: arXiv:2409.19771 source file (2025-05-08)
Supplement: Supplementary file 1 [file appendix.tex]

\appendices 
\section{Wheelchair Robot Details}
The wheelchair used is a Top End Pro Tennis wheelchair, motorized for autonomous control. A chain-drive system delivers power from the motors to the wheels. Each wheel is powered by a motor coupled to a 1:10 ratio speed-reducer planetary gearbox. The gearbox output shaft is connected to the wheel through a chain and sprocket system, providing an additional 1:2 speed reduction, resulting in a total reduction of 1:20. At maximum motor speed, the wheelchair can achieve linear velocities of up to 10 m/s and an in-place angular yaw velocity of up to 20 rad/s. Localization is achieved using wheel encoders, an IMU, and a Velodyne lidar sensor. The testing area is mapped beforehand, and sensor readings are used to localize the wheelchair within the map. For control, the system publishes commanded twist values, which are translated to left and right wheel velocities and tracked by a low-level PID controller at 200 Hz.

\section{Dataset Creation and Visualizations}
In this paper, we design an image processing pipeline to track the ball and the wheelchair in video footage. This section provides more details about the automatic dataset creation process and some of the issues detected.

\subsection{Details of Automatic Dataset Creation}
The objective of this phase is to extract useful data on player movements during gameplay to create a dataset suitable for model training. We began with videos of nine wheelchair tennis singles matches from the Tokyo 2020 Paralympic Games. The process involved six stages: (1) training a neural network to identify ball hit audio segments, (2) training a mean-shift model to identify non-matchplay segments, (3) obtaining court homography, (4) locating the tennis ball, (5) locating the closest player, and (6) combining aggregated data for training output.

\textbf{Model for Matchplay Detection:}
The video-based model uses a Mean Shift clustering algorithm to classify frames as either valid or invalid. Valid frames include a full overhead view of the tennis court, essential for collecting data on player movements and responses, while invalid frames show players recovering, commentators, detailed scoresheets, and crowd views. The model was trained on manually labeled video frames, preprocessed with resizing, Gaussian filtering, grayscale conversion, and intensity rescaling to enhance accuracy. The Mean Shift algorithm was applied to the feature vectors of the training data to learn the underlying clusters, identifying one cluster for valid frames and others for variations of invalid frames. \zz{The model achieved an accuracy of 99.62\% and an F-score of 99.63\% on the test dataset.}

\textbf{Model for Hit Detection:}
An audio-based model was trained to detect hits by identifying audio segments containing sounds resembling a player hitting the ball. Hit sounds are distinctive, while other match sounds include commentary, ball bounces, and typical match noise. The model architecture is a sequential neural network with dense layers and dropout regularization, processing audio segments using mel-frequency cepstral coefficients (MFCCs), chromagrams, and mel-spectrograms to create a flattened feature vector.

For training, we manually labeled timestamps of player hits in a small segment of a match, isolated the corresponding audio clips for hits, and selected non-overlapping segments for non-hits. The model, trained with categorical cross-entropy loss, achieved an accuracy of 92.3\%, effectively identifying timestamps for hits.

We initially used visual heuristics to detect changes in ball movement but found that audio extraction was more reliable due to unclear views and perspective distortion in broadcast videos. These visual challenges, particularly on the far side of the court, often led our algorithm to misinterpret the ball hitting the net as a successful return. As a result, generating accurate training data became difficult, and even TrackNet struggled to track the ball in such conditions consistently.

\subsection{Video Processing Visualization}
Here, we visualize the success and failure modes of ball and wheelchair detection to better explain our experimental results. The failure modes mainly include ball detection failure, wheelchair detection failure, and hit detection failure, as shown in Figure \ref{fig:dataset_failure}.

\begin{figure}
     \centering
     \begin{subfigure}[b]{0.47\columnwidth}
         \centering
         \includegraphics[width=\textwidth]{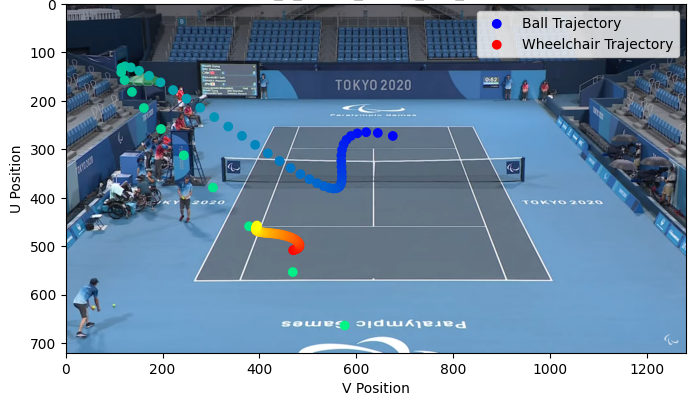}
         \caption{Tennis detection failure}
         \label{fig:ball}
         \vspace{1em}
     \end{subfigure}
     \begin{subfigure}[b]{0.47\columnwidth}
         \centering
         \includegraphics[width=\textwidth]{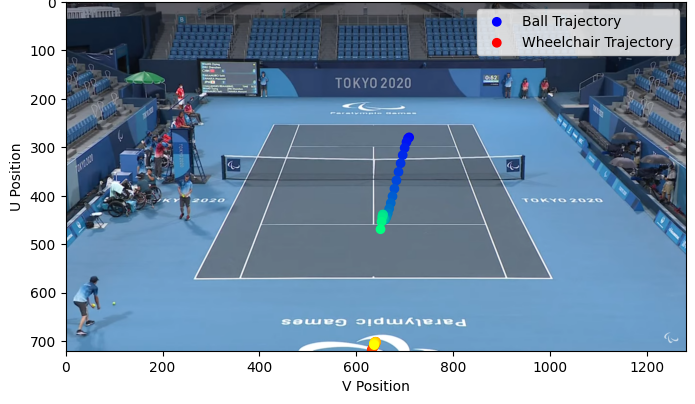}
         \caption{Wheelchair detection failure}
         \label{fig:wheelchair}
         \vspace{1em}
     \end{subfigure} 
    
    \begin{subfigure}[b]{0.47\columnwidth}
         \centering
         \includegraphics[width=\textwidth]{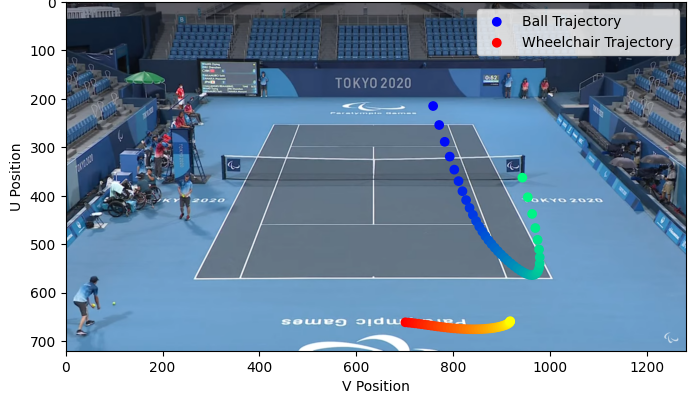}
         \caption{Hit detection Failure}
         \label{fig:hit}
     \end{subfigure}
    \begin{subfigure}[b]{0.47\columnwidth}
         \centering
         \includegraphics[width=\textwidth]{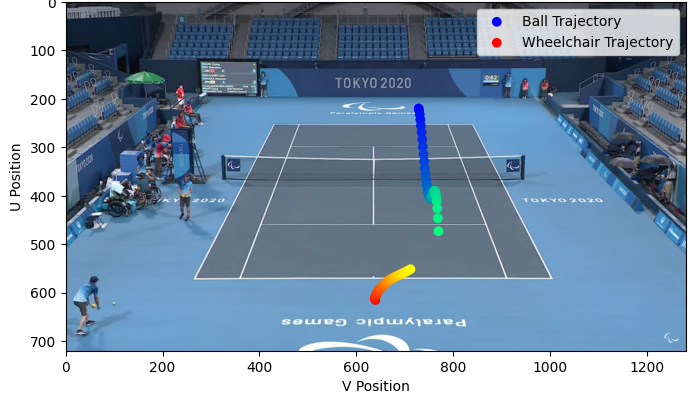}
         \caption{Success}
         \label{fig:success}
     \end{subfigure}
        \caption{Dataset visualizations: failure modes and success.}
        \label{fig:dataset_failure}
\end{figure}

From Figure \ref{fig:ball}, we observe that the algorithm sometimes mistakenly identifies an object in the audience as the tennis ball, causing the trajectory to bend towards it. Figure \ref{fig:wheelchair} shows a failure in wheelchair detection where the algorithm misidentifies the Paralympics pattern as the wheelchair. Additionally, Figure \ref{fig:hit} shows that the racket-ball hitting point is sometimes not well estimated, resulting in incorrectly cut trajectories that include part of the return. Conversely, Figure \ref{fig:success} demonstrates successful detection and tracking of the ball and wheelchair, as well as accurate hit detection, highlighting the pipeline's potential effectiveness when operating correctly. \zz{Our policy achieves improved performance when a human identifies and removes flawed or problematic trajectories from the training dataset.}
% Our policy can perform better when we manually extract the successful trajectory parts in the training dataset.

\section{Imitation Learning Model Parameters} \label{sec:parameter}
In this section, we present the training parameters of the imitation learning models used in our study. The prediction horizon ($L_p$) indicates the total number of waypoints that the model predicts for the path per inference. The history length ($L_h$) is the number of the observed trajectory points based on which we are predicting the future. See Table \ref{tab:diffusion}-\ref{tab:ae_mlp} for the hyperparameters we use for each imitation policy.

\begin{table}[h]
\centering
\begin{minipage}[b]{0.48\columnwidth}
\centering
\caption{Diffusion}
\label{tab:diffusion}
\resizebox{\textwidth}{!}{
\begin{tabular}{lcc}
\hline
Parameter Name  & Notation & Value \\ \hline
Learning rate   & $l_d$    & 2e-5  \\
Weight decay    & $wd$     & 0  \\
Prediction horizon    & $L_p$    & 18   \\ 
History length    & $L_h$    & 32   \\ 
Epoch number    & $N_d$    & 1000   \\ \hline
\end{tabular}
}
\vspace{4mm}
\end{minipage}%
\begin{minipage}[b]{0.48\columnwidth}
\centering
\caption{ACT}
\label{tab:act}
\resizebox{\textwidth}{!}{
\begin{tabular}{lcc}
\hline
Parameter Name  & Notation & Value \\ \hline
Learning rate   & $l_d$    & 1e-5  \\
Weight decay    & $wd$     & 0  \\
Prediction horizon    & $L_p$    & 18   \\ 
History length    & $L_h$    & 32   \\ 
Epoch number    & $N_d$    & 200   \\ \hline
\end{tabular}
}
\vspace{4mm}
\end{minipage}

\begin{minipage}[b]{0.48\columnwidth}
\centering
\caption{FCR}
\label{tab:mlp}
\resizebox{\textwidth}{!}{
\begin{tabular}{lcc}
\hline
Parameter Name  & Notation & Value \\ \hline
Learning rate   & $l_d$    & 1e-3  \\
Weight decay    & $wd$     & 0  \\
Prediction horizon    & $L_p$    & 18   \\ 
History length    & $L_h$    & 32   \\ 
Epoch number    & $N_d$    & 1000   \\ \hline
\end{tabular}
}
\end{minipage}%
\begin{minipage}[b]{0.48\columnwidth}
\centering
\caption{AE-FCR}
\label{tab:ae_mlp}
\resizebox{\textwidth}{!}{
\begin{tabular}{lcc}
\hline
Parameter Name  & Notation & Value \\ \hline
Learning rate   & $l_d$    & 1e-3  \\
Weight decay    & $wd$     & 0.75  \\
Prediction horizon    & $L_p$    & 18   \\ 
History length    & $L_h$    & 32   \\ 
Epoch number    & $N_d$    & 500 \\ \hline
\end{tabular}
}
\end{minipage}
\end{table}

\section{Physical Robot Experiment Details}
In this section, we introduce the details of our real-world experiments. 

\subsection{Vision System}
To track and detect the tennis ball, we employ a multi-camera setup. The system consists of six Blackfly S cameras, each connected to a Jetson Xavier. The cameras are mounted on the back walls of the court at a height of 5.5 meters, looking down at the court. Three cameras are mounted on each side of the court, providing overlapping coverage of the entire court (Figure~\ref{fig:camera_real_setting}). This setup maximizes the chances of detecting the ball with multiple cameras and allows us to track the ball from various angles, making the system more robust than using cameras from the same angle. The Jetsons detect the ball in the images and share the detections over Ethernet to a central computer that computes the ball state (location and velocity) based on detections from different cameras. To estimate the dynamic states of the tennis ball—position, velocity, and spin—we utilize a factor graph that processes data asynchronously \cite{xiao2024multi}. This approach aggregates the detection results from all six cameras asynchronously and publishes accurate estimation and prediction of the states. For real-time performance in inference, the GTSAM package \cite{gtsam}, which is based on the ISAM2 algorithm \cite{kaess2012isam2}, is employed. The inference and prediction speed in total is about 300 Hz, which is sufficient for our real time experiments.
\begin{figure}[h]
    \vspace{-4mm}
    \centering
    \includegraphics[width=0.99\columnwidth]{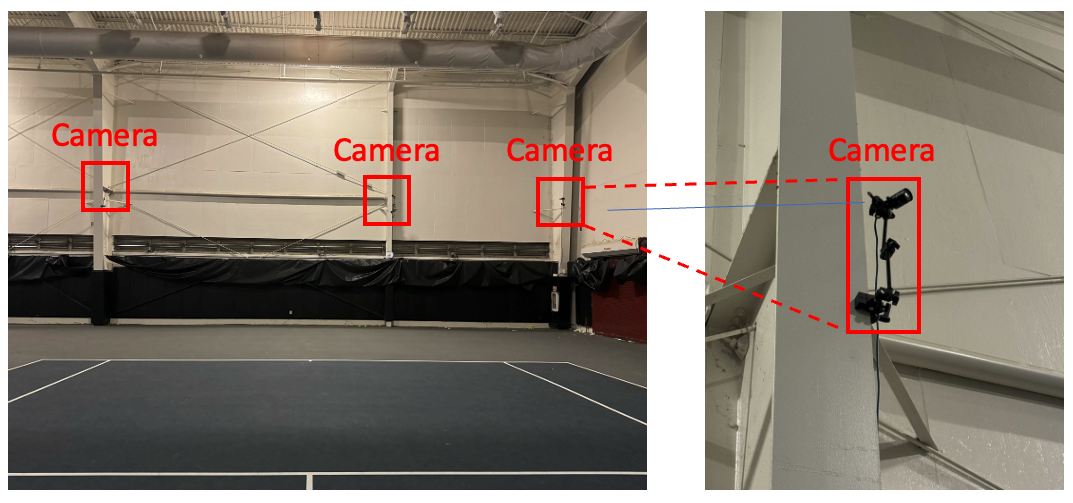}
    \caption{Camera configurations in the real court: cameras are boxed and zoomed in.}
    \label{fig:camera_real_setting}
    \vspace{-5mm}
\end{figure}

\subsection{Hybrid Testing Details}

We conduct hardware-in-the-loop testing on a robotic wheelchair in an enclosed space, as shown in Figure~\ref{fig:ctrl_seq}. The \zz{real-world ball} trajectories from the collected dataset are replayed one by one, and the robot acts according to the control architecture shown in Figure~\ref{fig:control}. Our control system runs on the ROS framework, with ROS nodes distributed across two computers: a high-performance workstation and an on-board PC (NUC). These computers communicate over WiFi, exchanging information through ROS topics.
\begin{figure*}[h]
     \centering
     \begin{subfigure}[b]{0.19\textwidth}
         \centering
         \includegraphics[width=\textwidth]{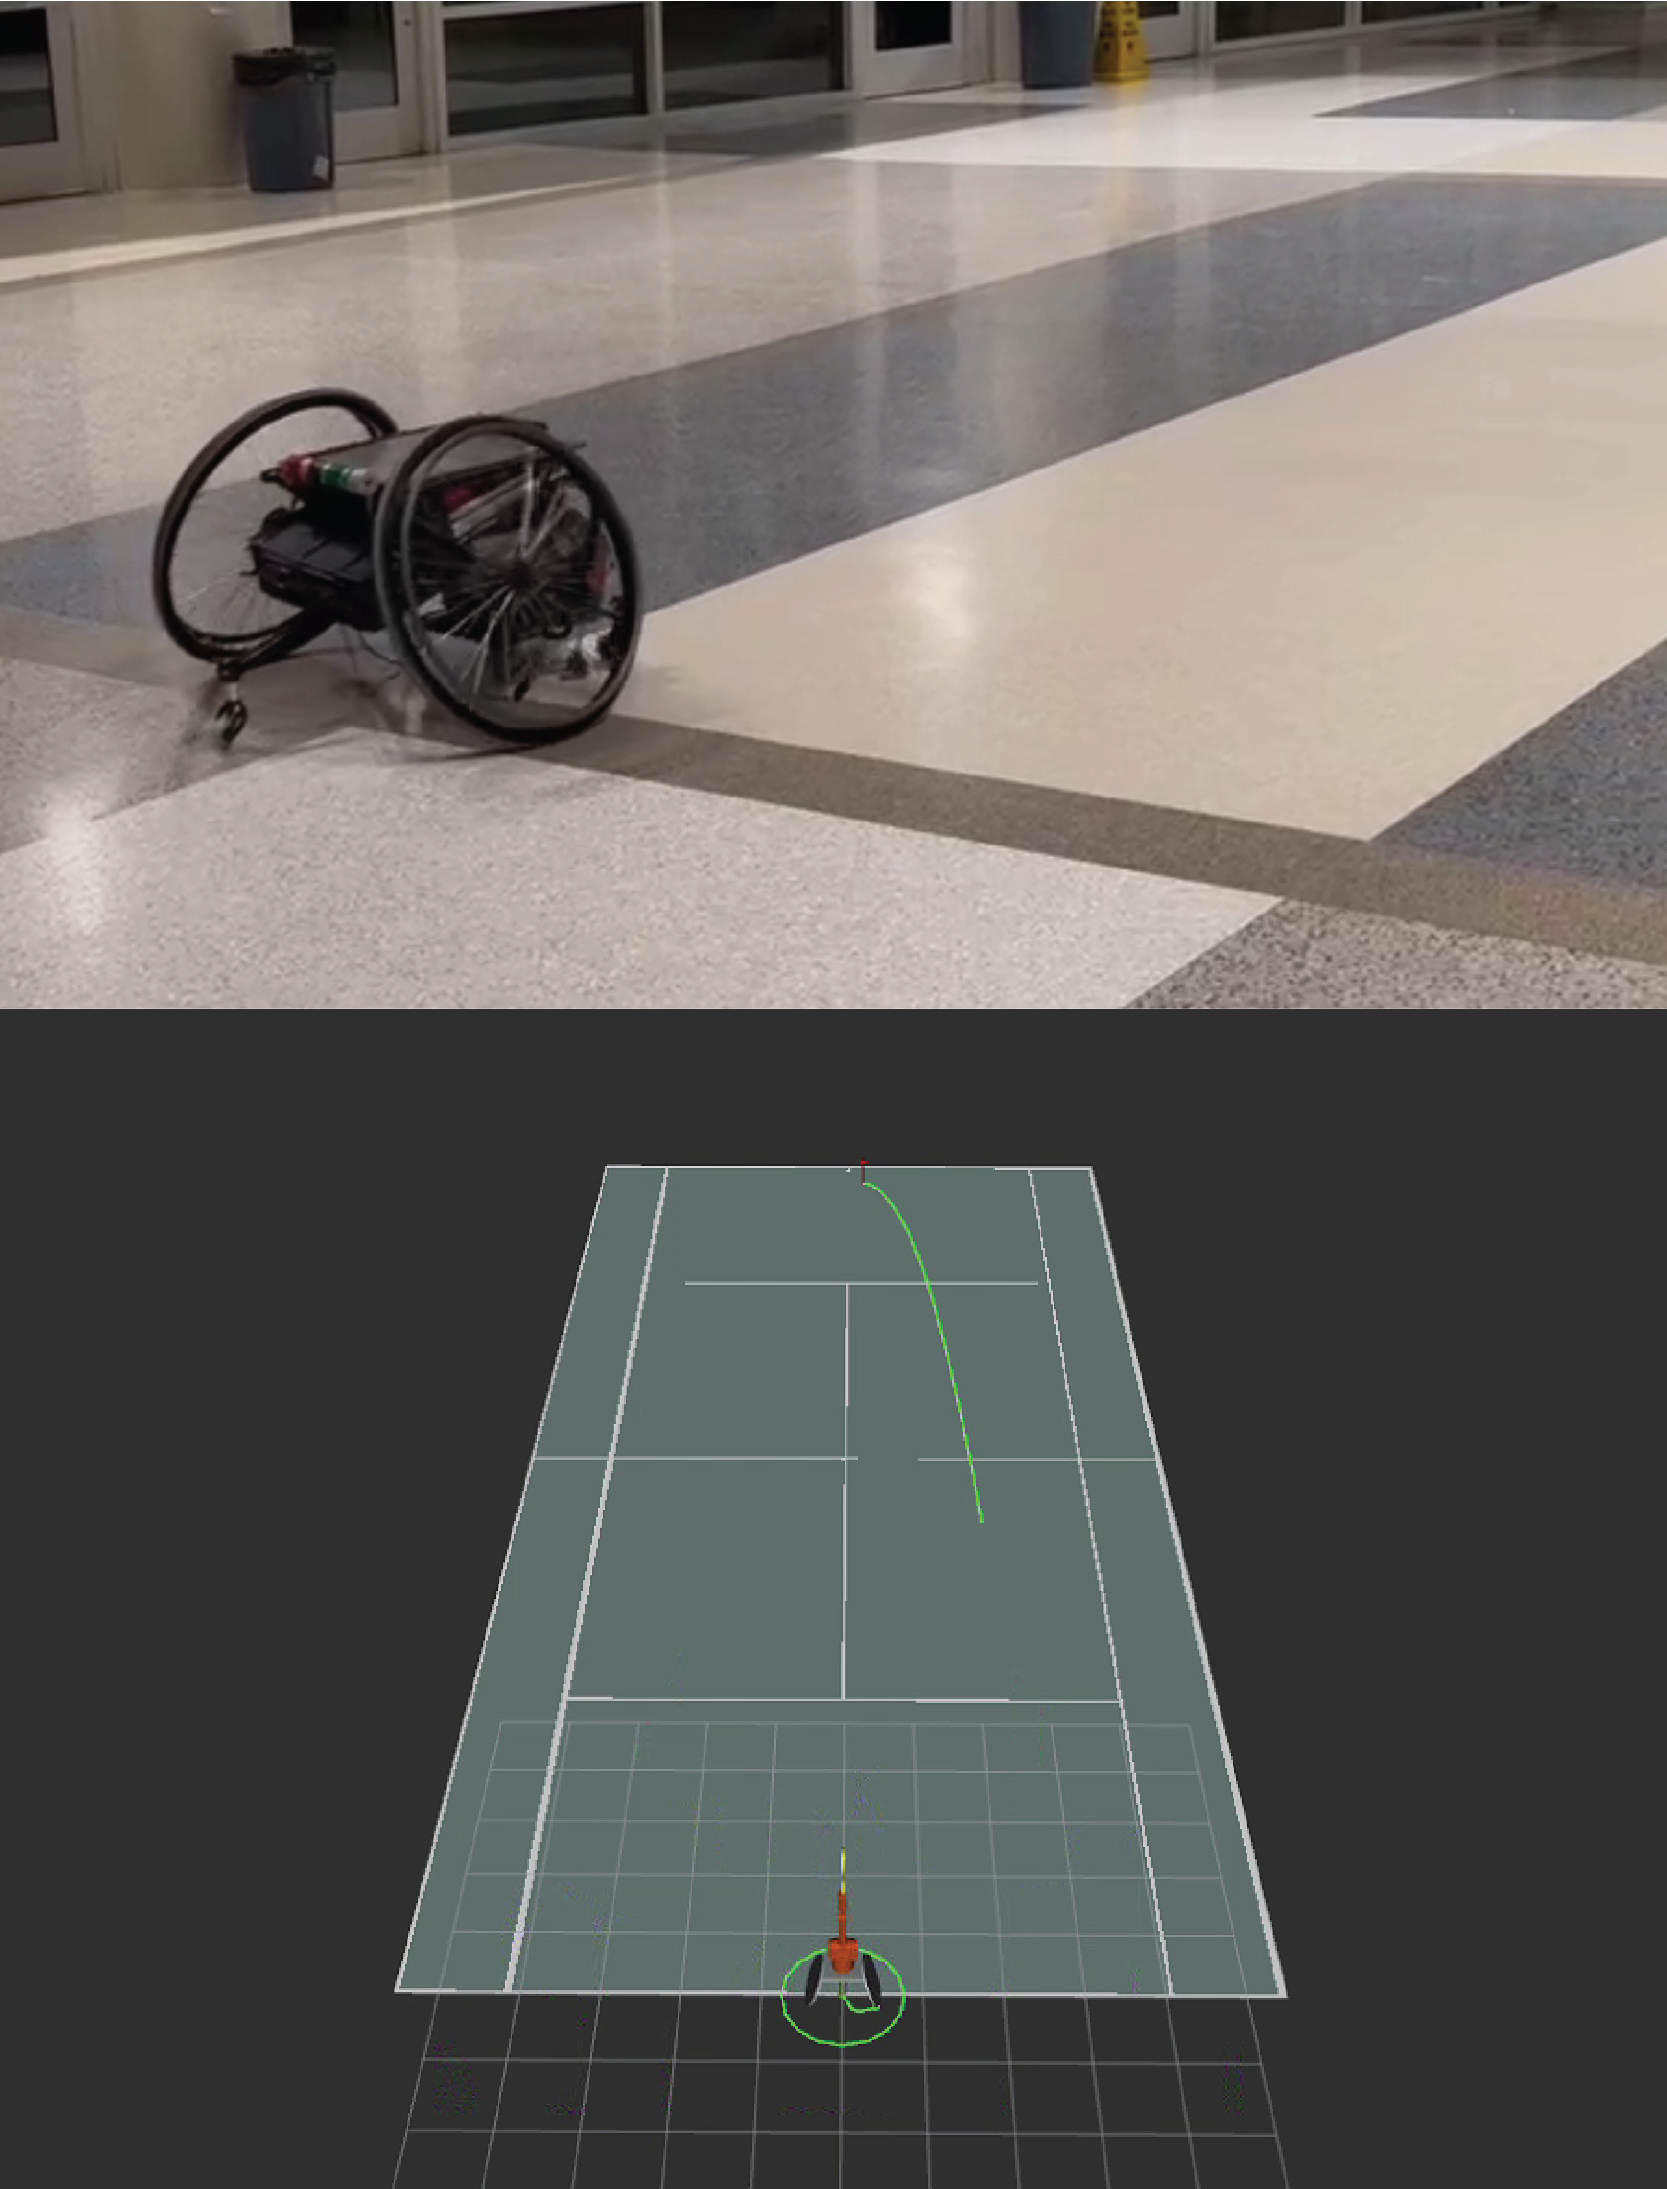}
         \caption{}
         \label{fig:ctrl_s}
     \end{subfigure}
     \begin{subfigure}[b]{0.19\textwidth}
         \centering
         \includegraphics[width=\textwidth]{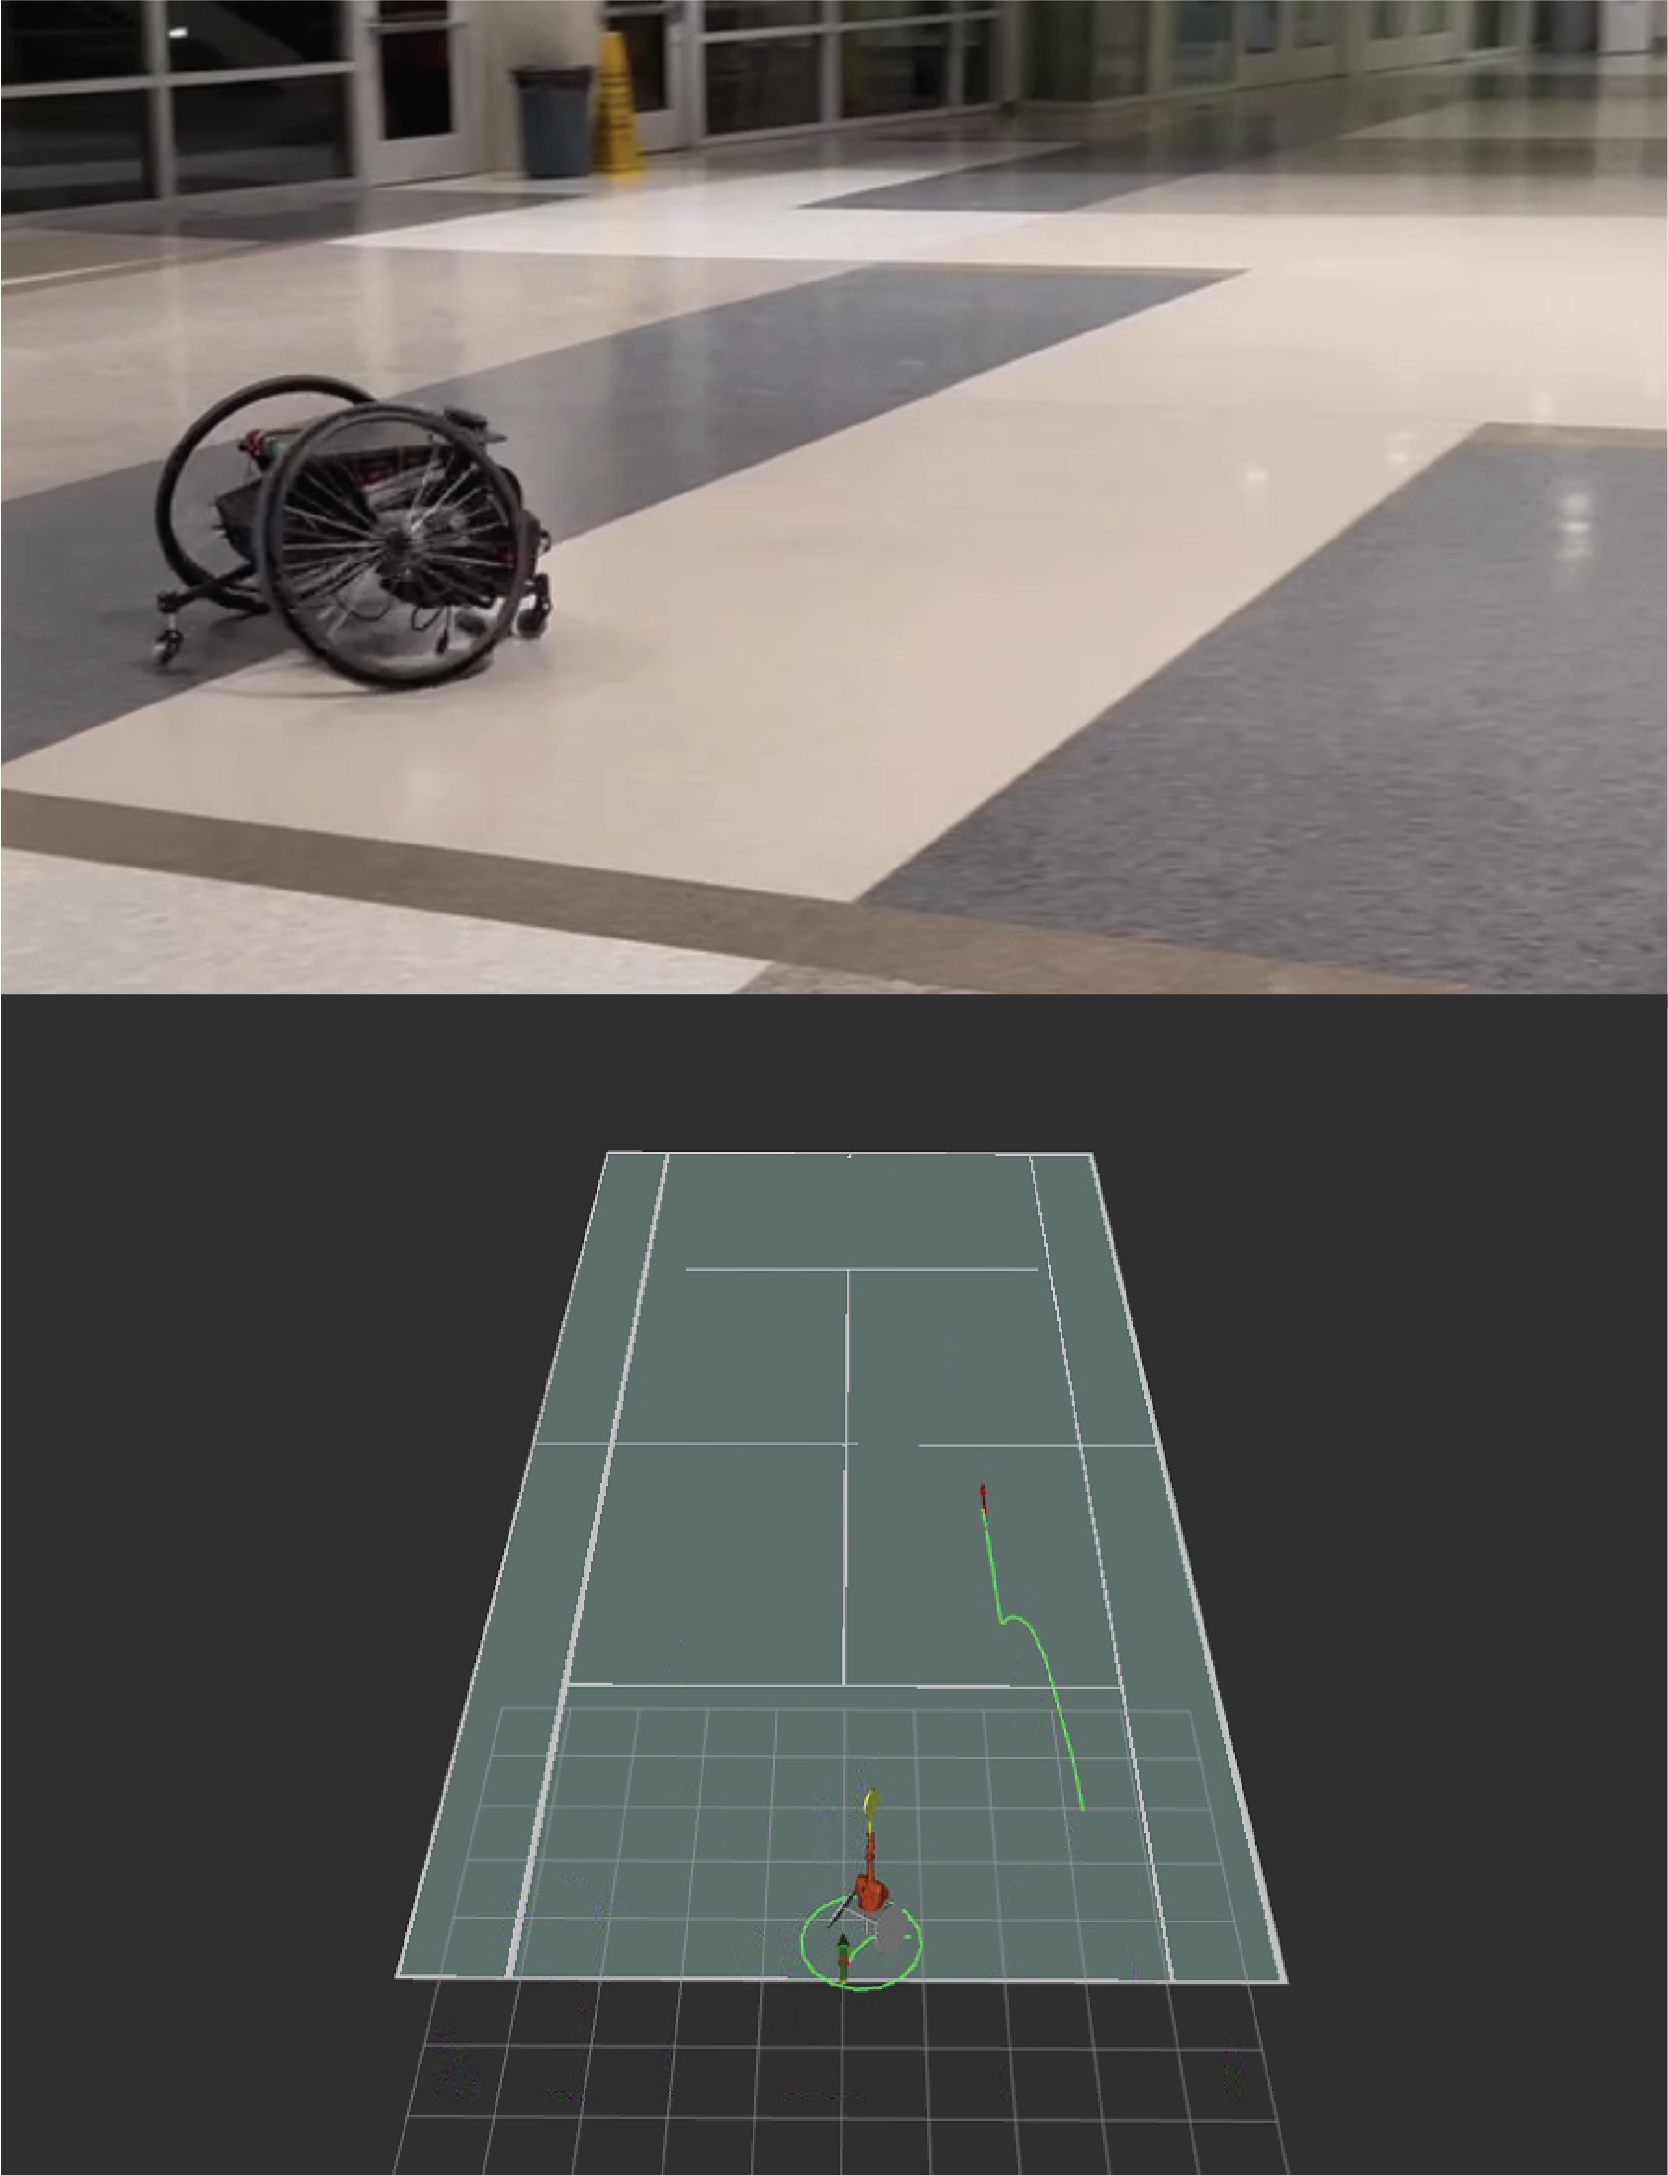}
         \caption{}
     \end{subfigure}
     \begin{subfigure}[b]{0.19\textwidth}
         \centering
         \includegraphics[width=\textwidth]{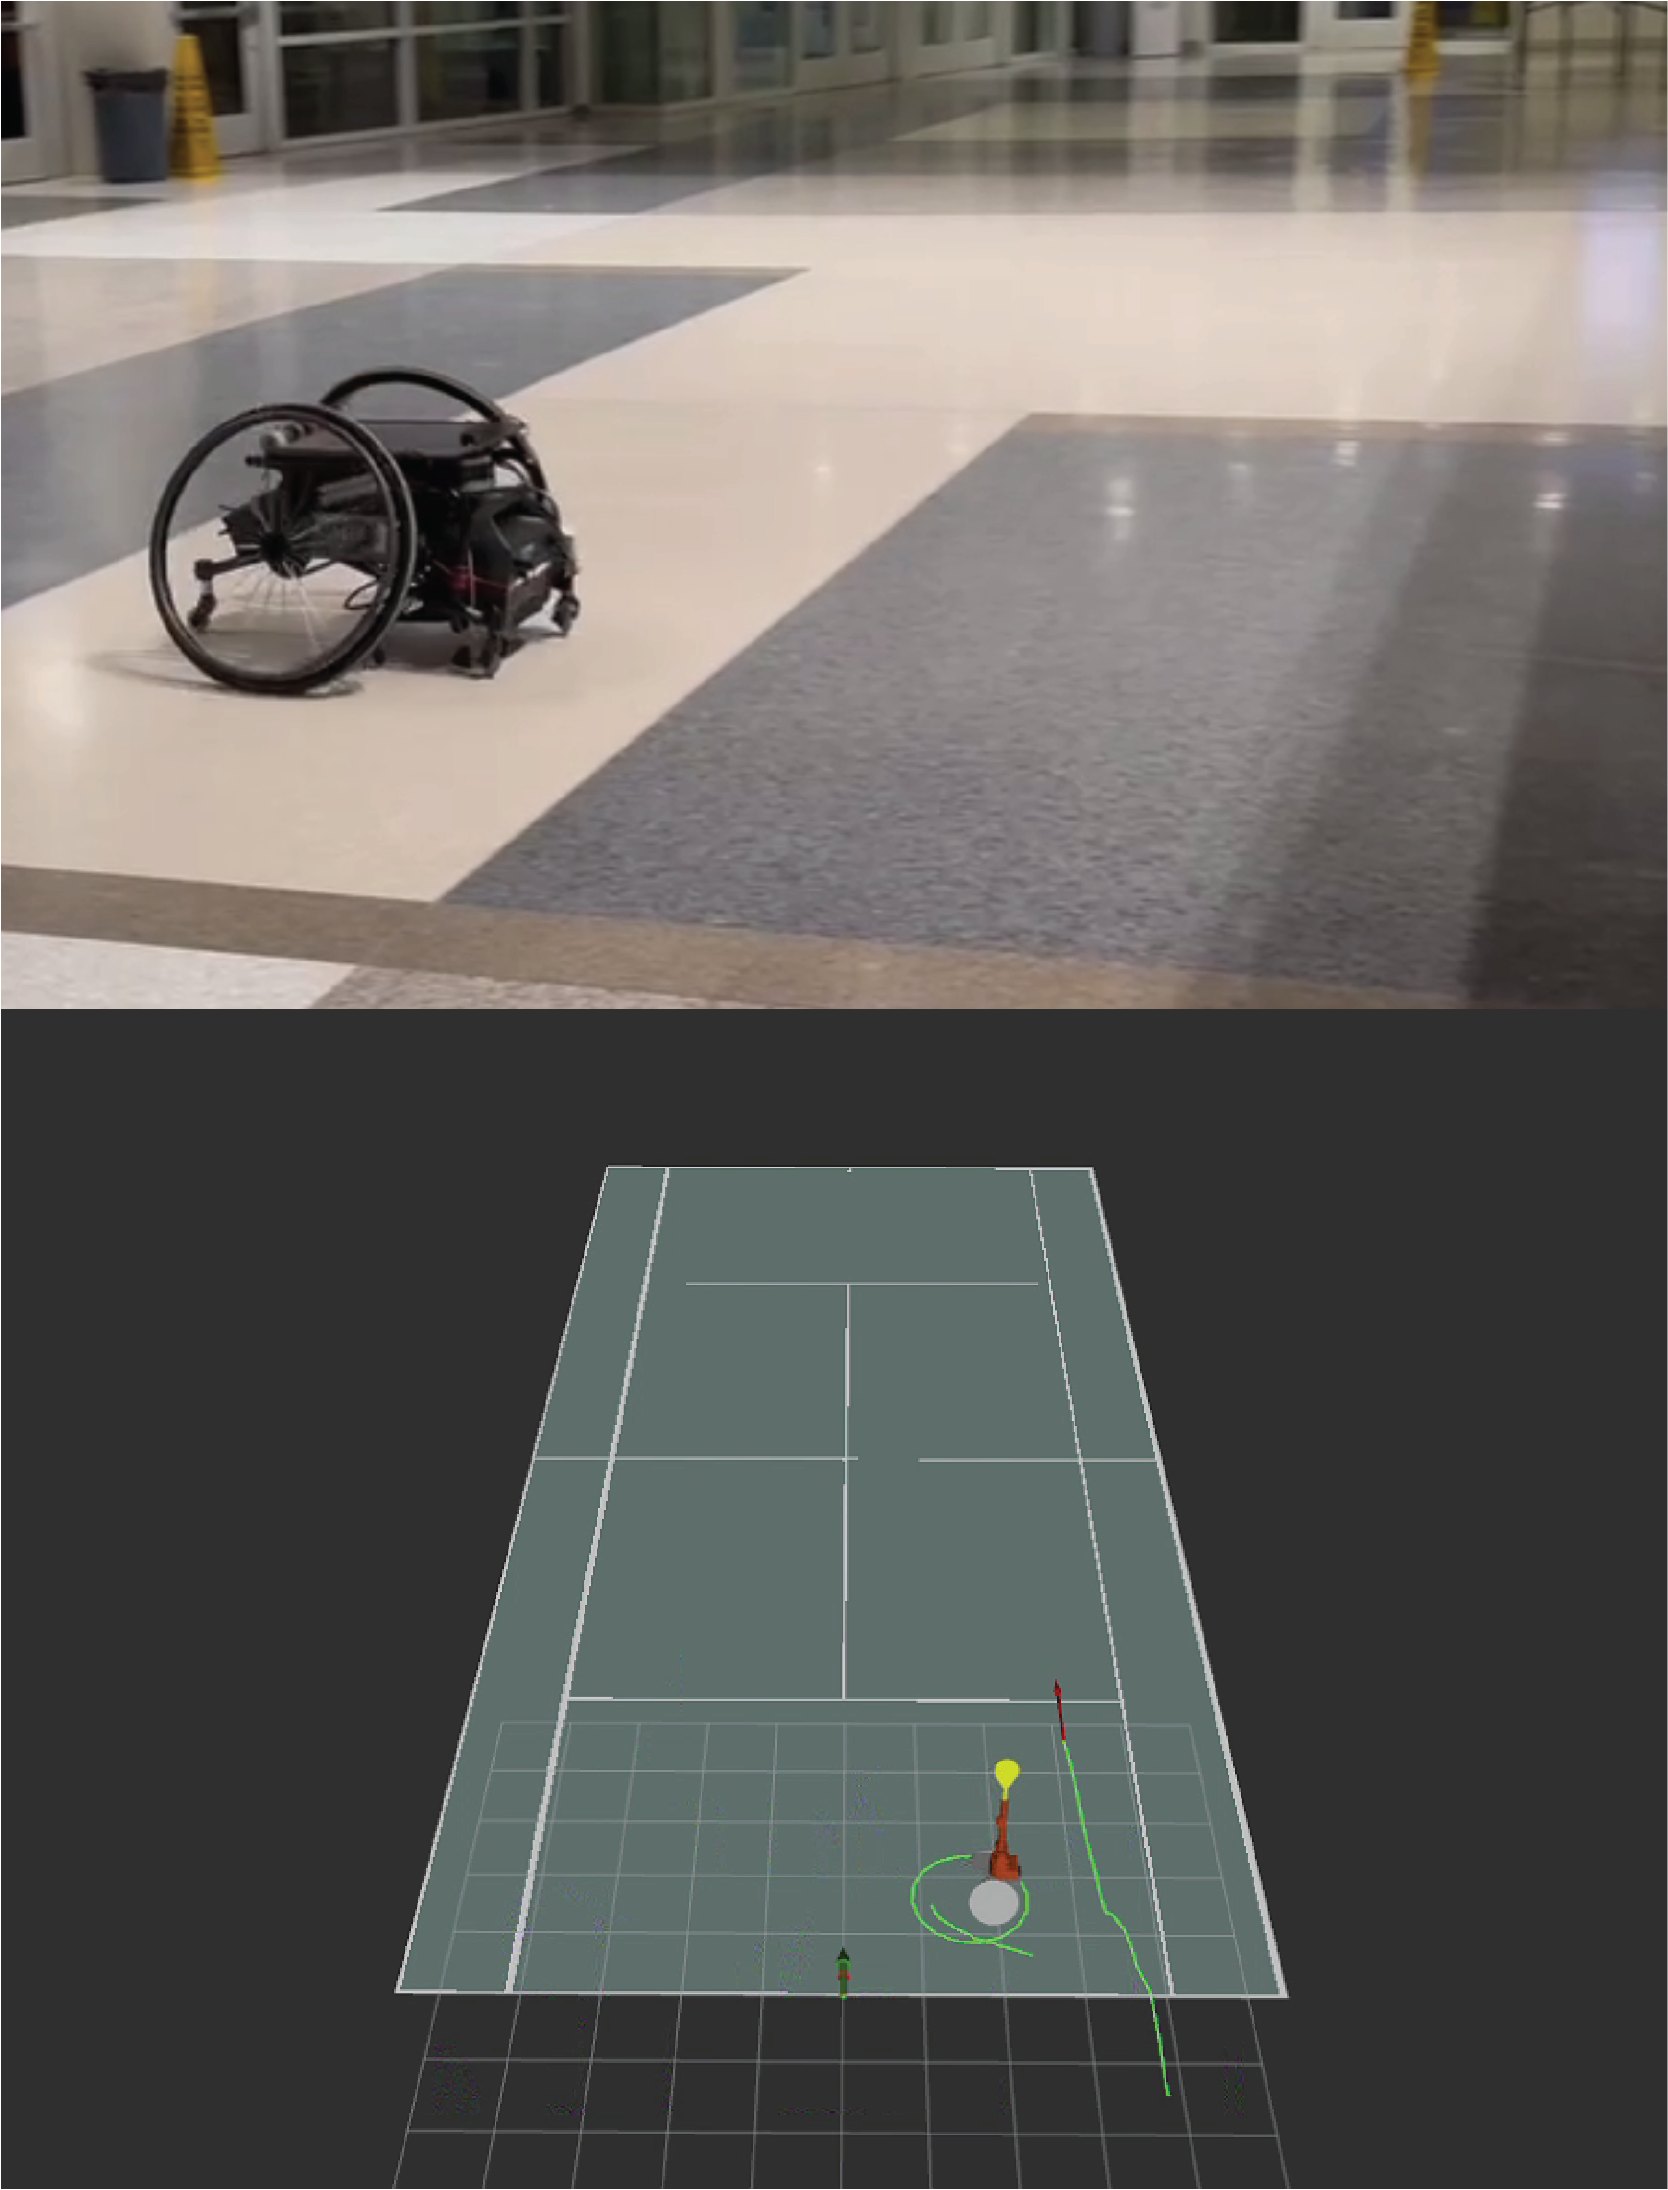}
         \caption{}
     \end{subfigure}
     \begin{subfigure}[b]{0.19\textwidth}
         \centering
         \includegraphics[width=\textwidth]{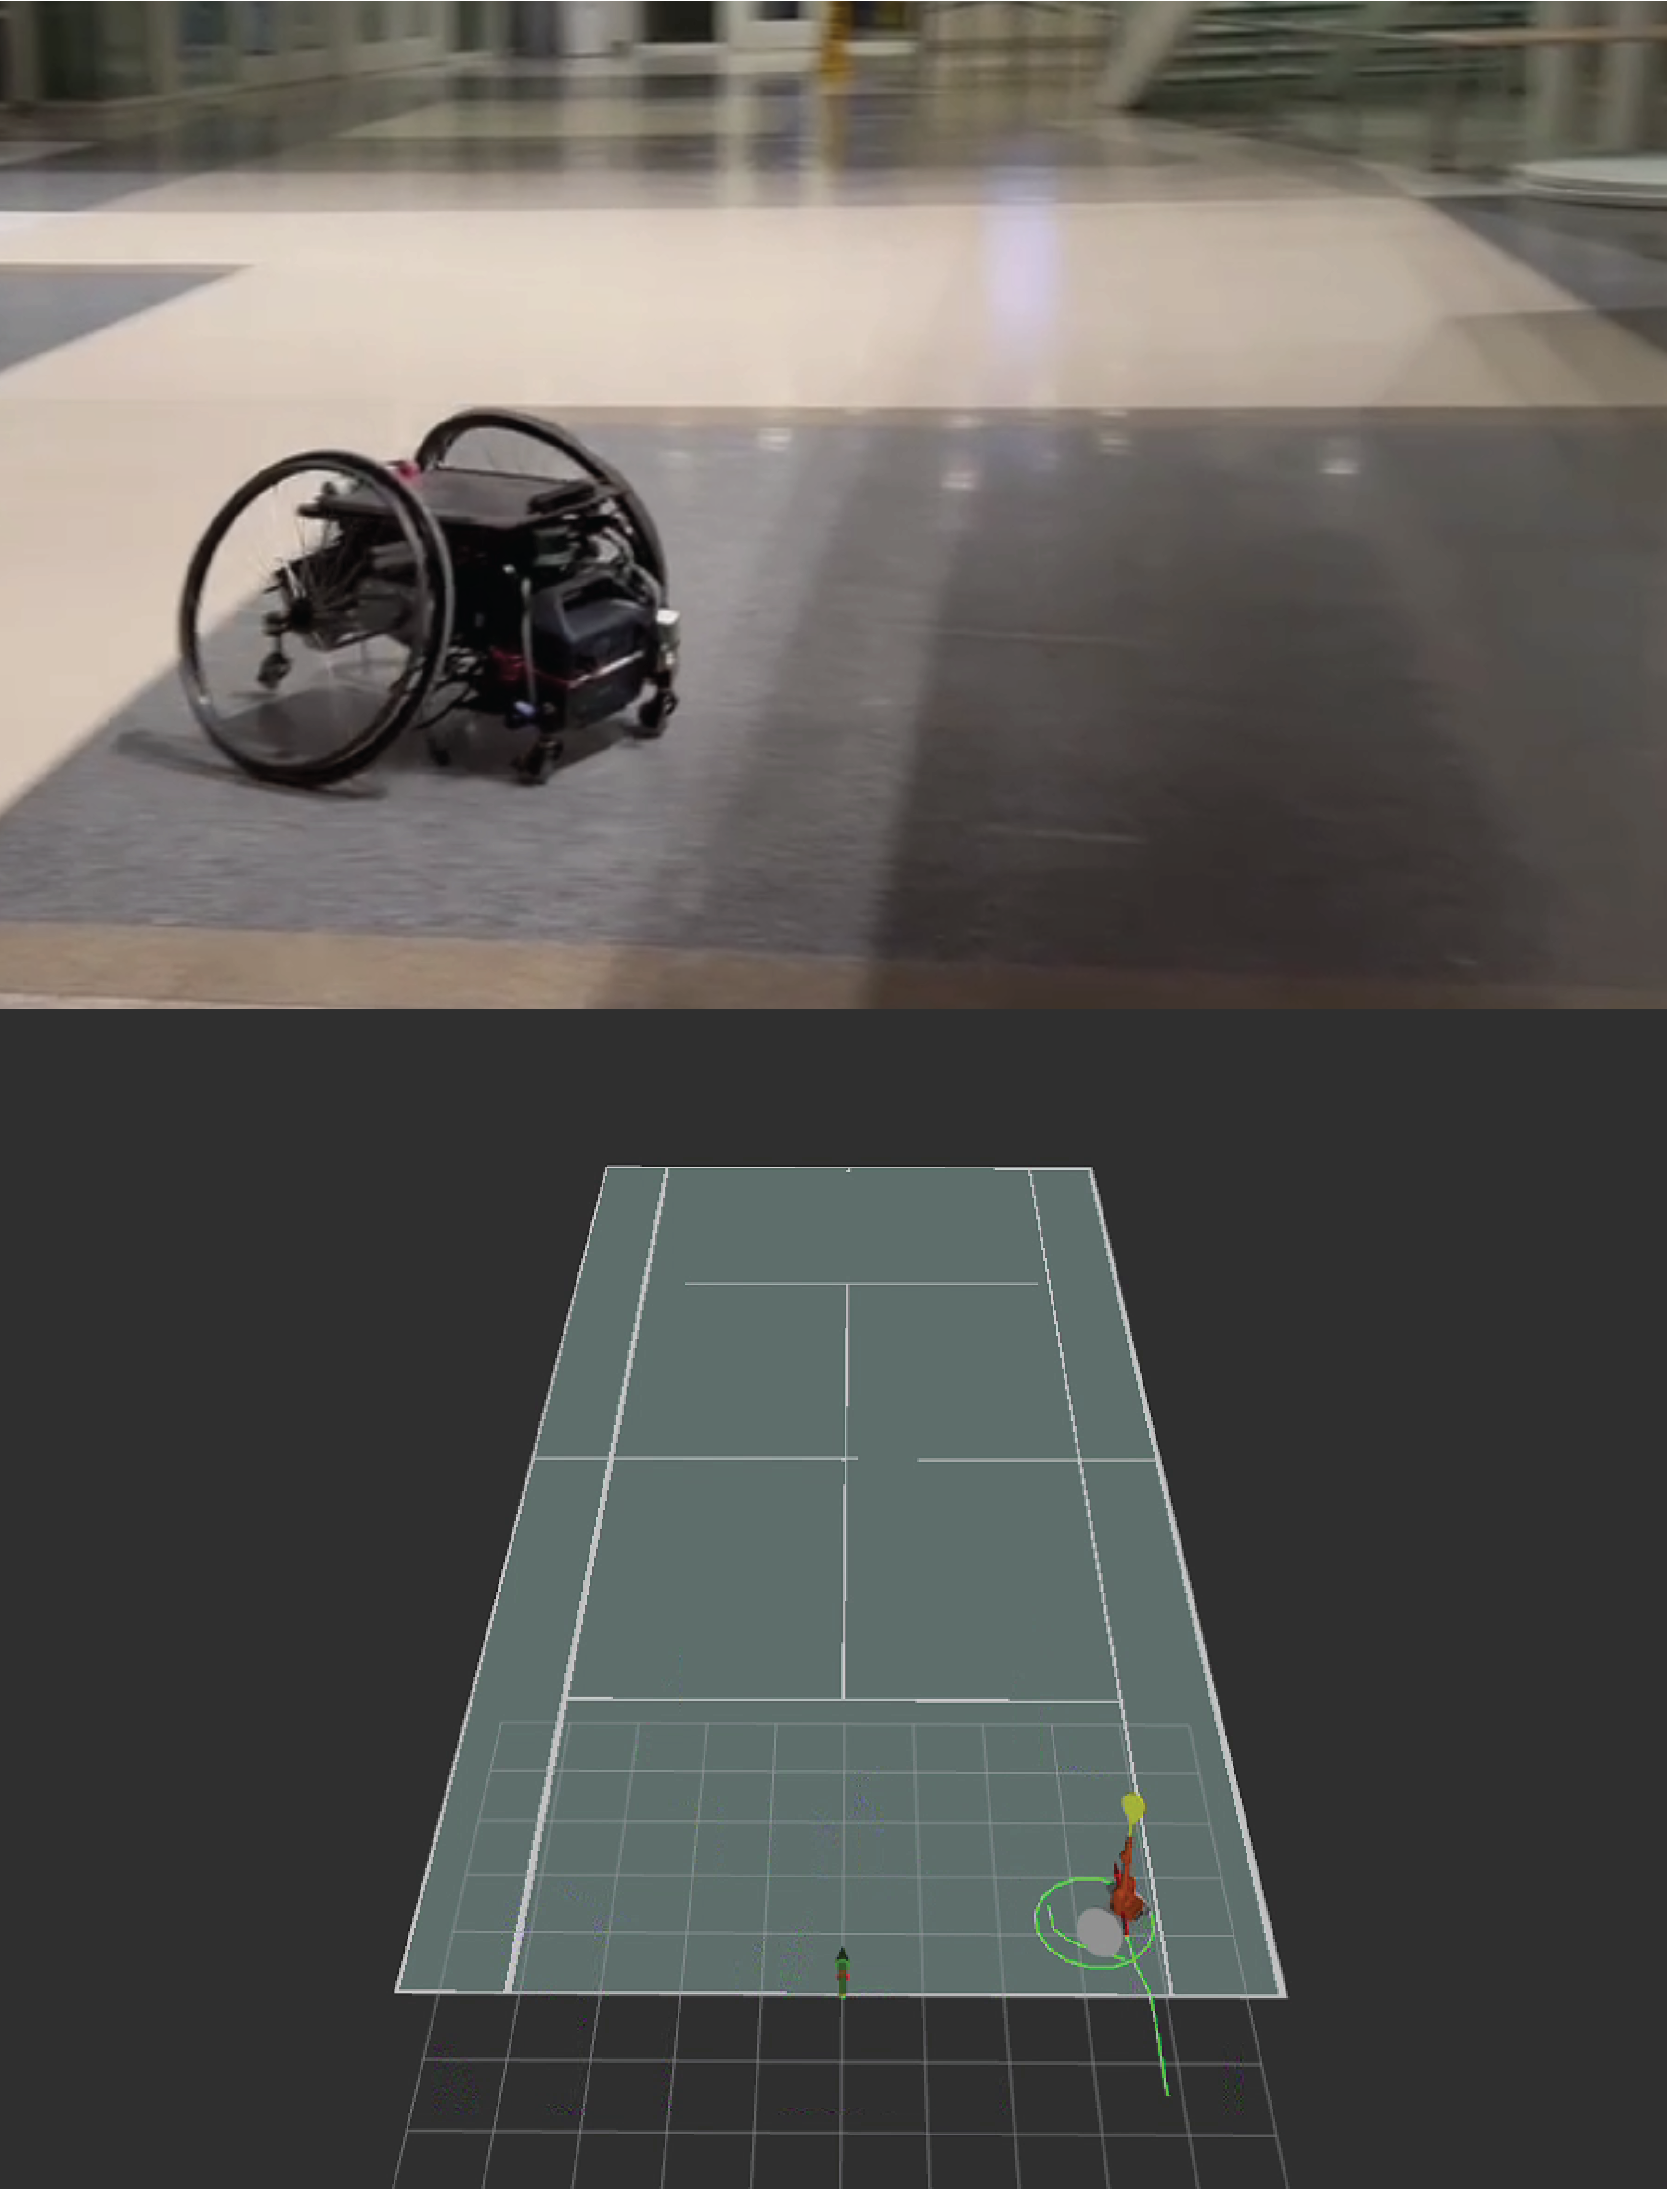}
         \caption{}
     \end{subfigure}
     \begin{subfigure}[b]{0.19\textwidth}
         \centering
         \includegraphics[width=\textwidth]{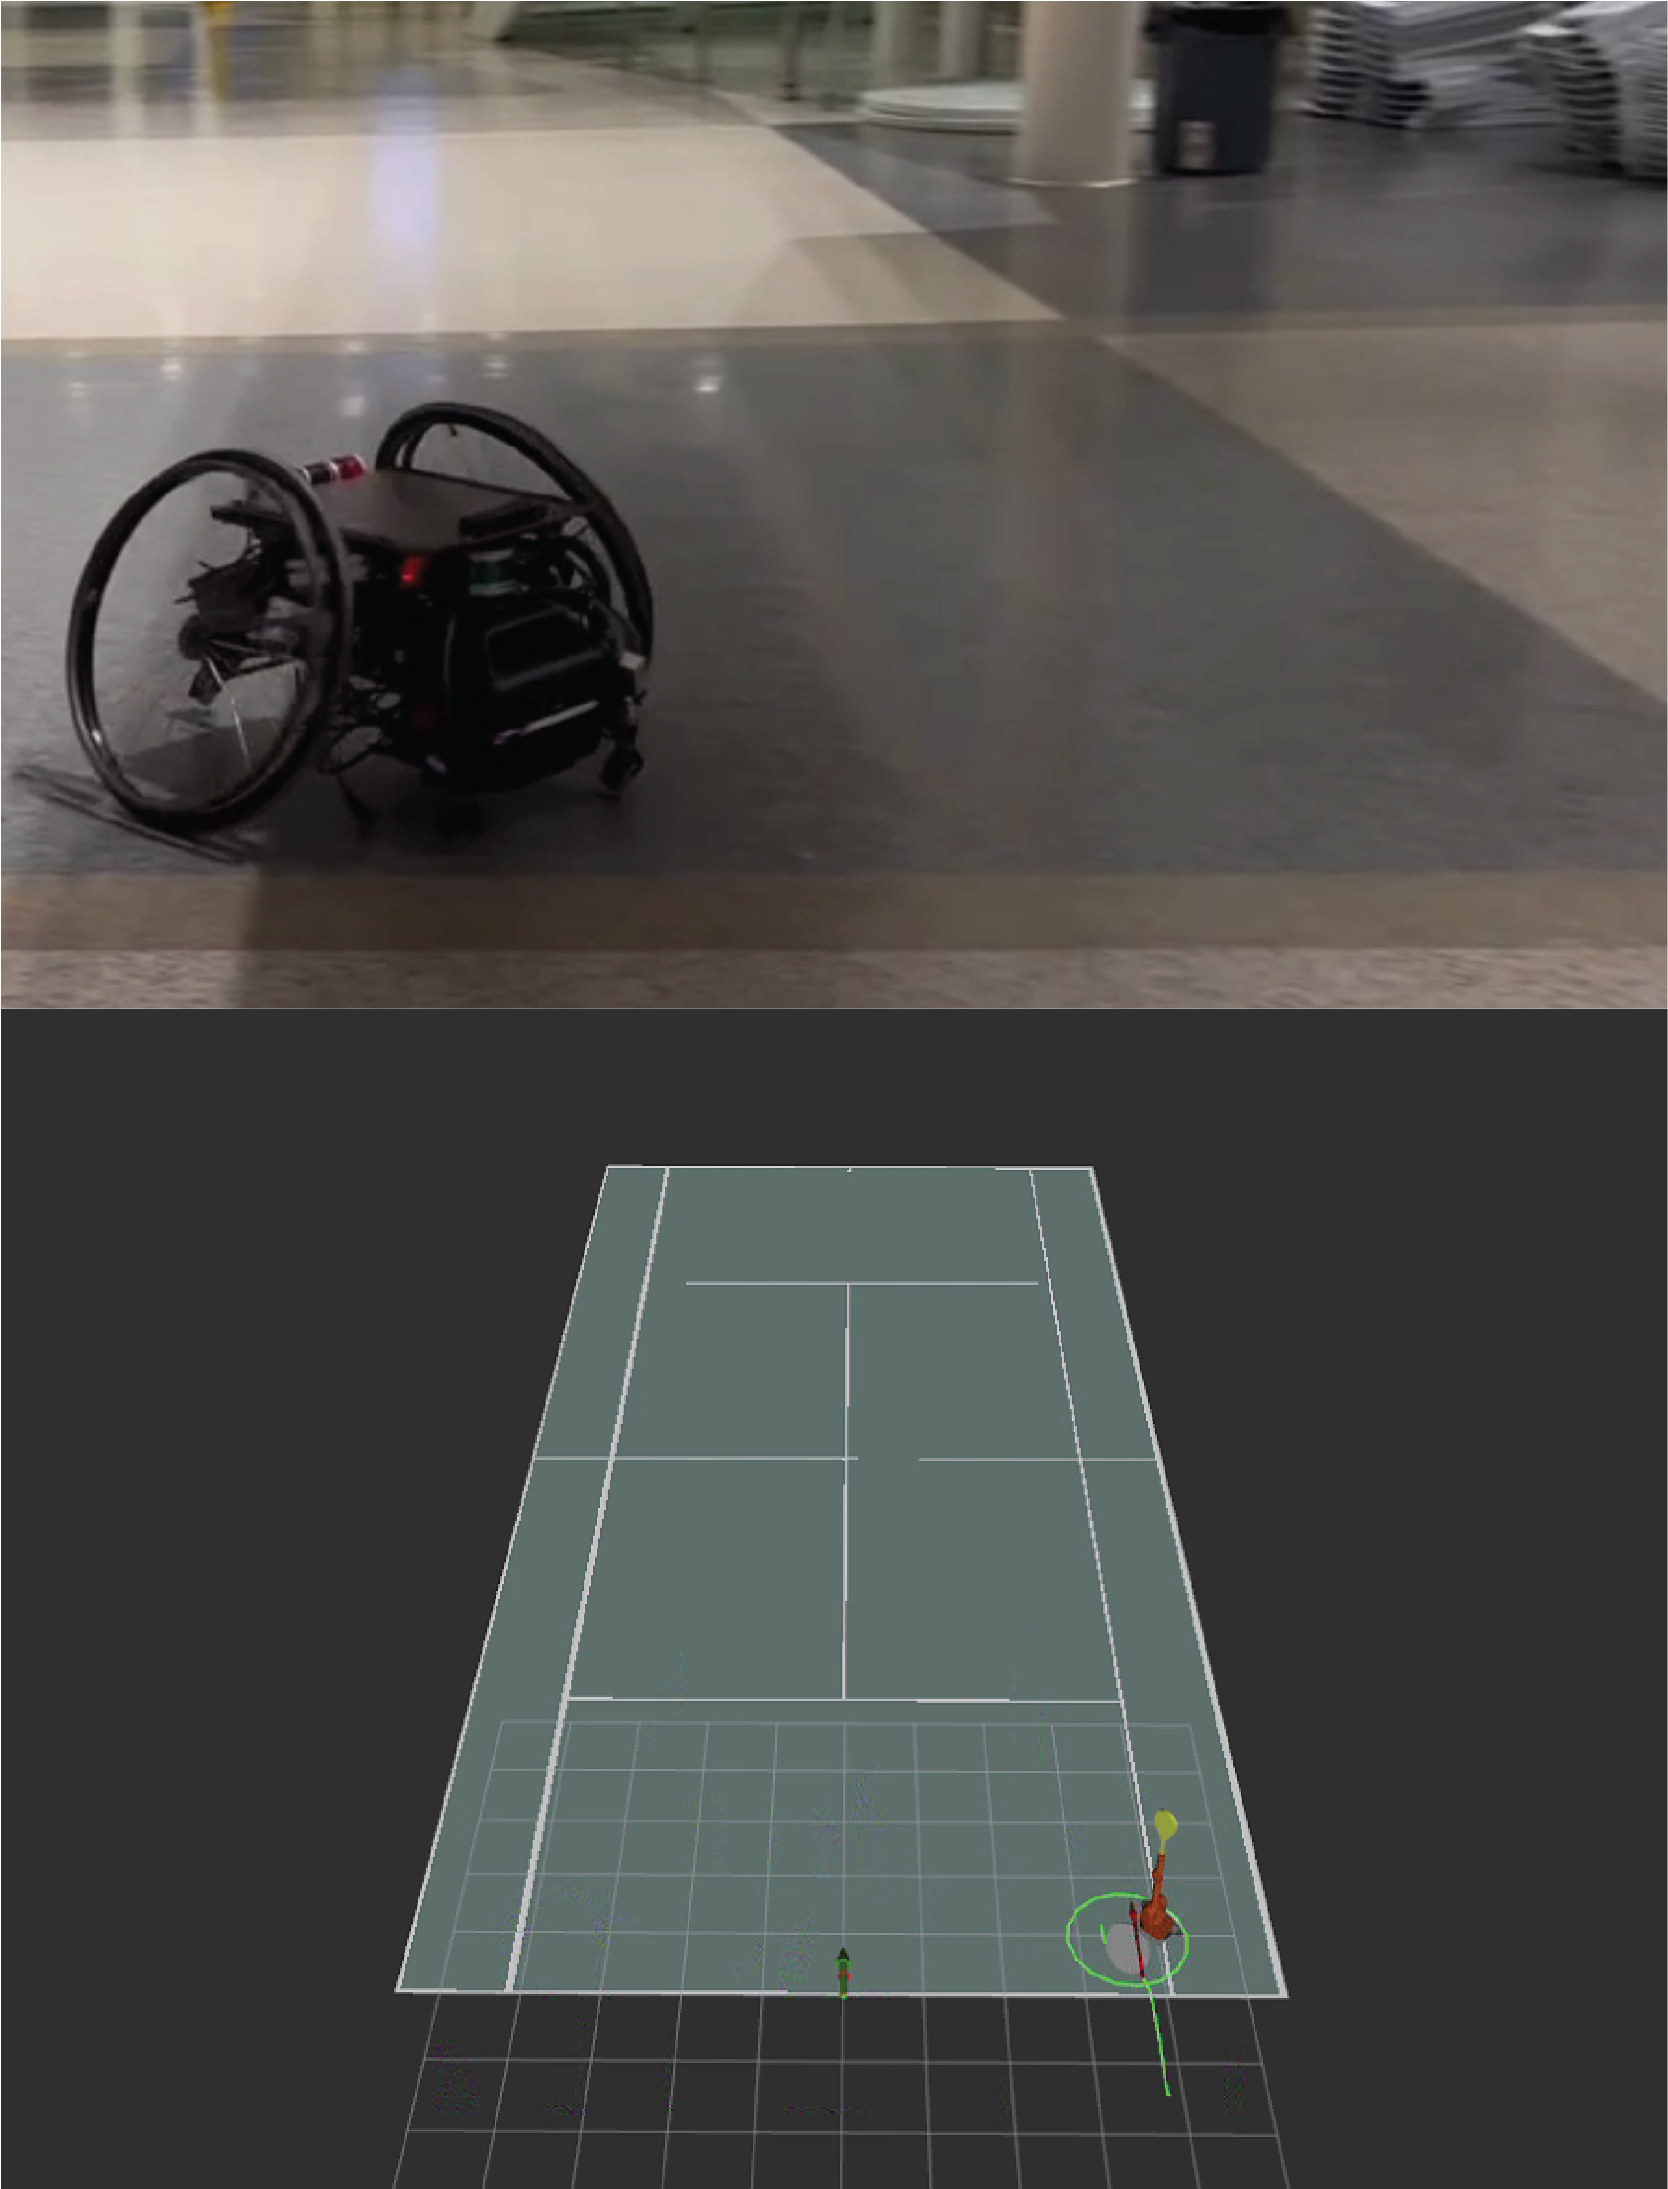}
         \caption{}
         \label{fig:ctrl_e}
     \end{subfigure}
        \caption{We visualize the hardware-in-the-loop experiment on the robotic wheelchair. The ball is launched to the right side of the court, and the robotic wheelchair successfully navigates to intercept the ball.}
        \label{fig:ctrl_seq}
\end{figure*}
\begin{figure}[ht]
    \centering
    \includegraphics[width=0.9\linewidth]{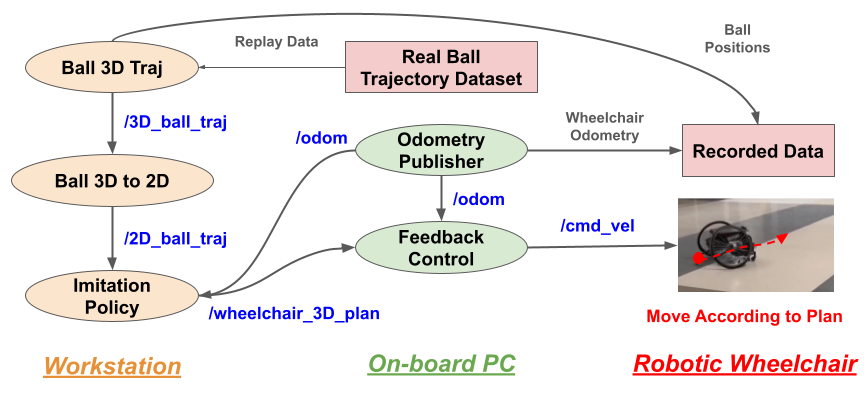}
    \caption{Control architecture for hardware-in-loop testing.}
    \label{fig:control}
    \vspace{-5mm}
\end{figure}
We run the imitation policy on the workstation due to its high computational requirements, which the on-board PC cannot handle. The imitation policy receives odometry information from the on-board PC and the ball trajectory converted to 2D image space, generating a local plan for the wheelchair. This local plan is then sent back to the on-board PC. The PD feedback controller on the on-board PC provides the command velocities based on the current odometry and the local plan. We record the wheelchair odometry data and the ball's 3D data, which can be post-processed to determine if the robotic wheelchair successfully intercepted the ball.

Figure \ref{fig:ctrl_seq} illustrates our imitation learning-based motion planner in action, combined with the real robot PD feedback control results. The top row shows the wheelchair in an enclosed space, while the bottom row displays the corresponding positions on the tennis court. The wheelchair starts from the center position of the baseline on the tennis court (shown in Figure \ref{fig:ctrl_s}) and navigates to intercept the ball served to the right side of the court (Figures \ref{fig:ctrl_s}-\ref{fig:ctrl_e}).

\section{Generalizability of Data Extraction Approach}
A contribution of our work is the development of an efficient, integrated pipeline that transforms raw broadcast tennis videos into data suitable for robot learning applications. To illustrate its effectiveness and flexibility, we adapted this pipeline to analyze table tennis gameplay. With minimal adjustments, we successfully repurposed our data extraction pipeline from broadcast tennis matches to table tennis. \zz{We were able to complete essential tasks, such as homography identification, player tracking, and ball tracking, much more quickly using broadcast footage from the recent Paris Olympics—a process that previously required extensive time and effort to optimize for tennis.}
% We were able to complete essential tasks, such as homography identification, player tracking, and ball tracking, within a few hours using broadcast footage from the recent Paris Olympics— a process that initially took months to optimize for tennis.

\begin{figure}[H]
\centering
\includegraphics[width=\columnwidth]{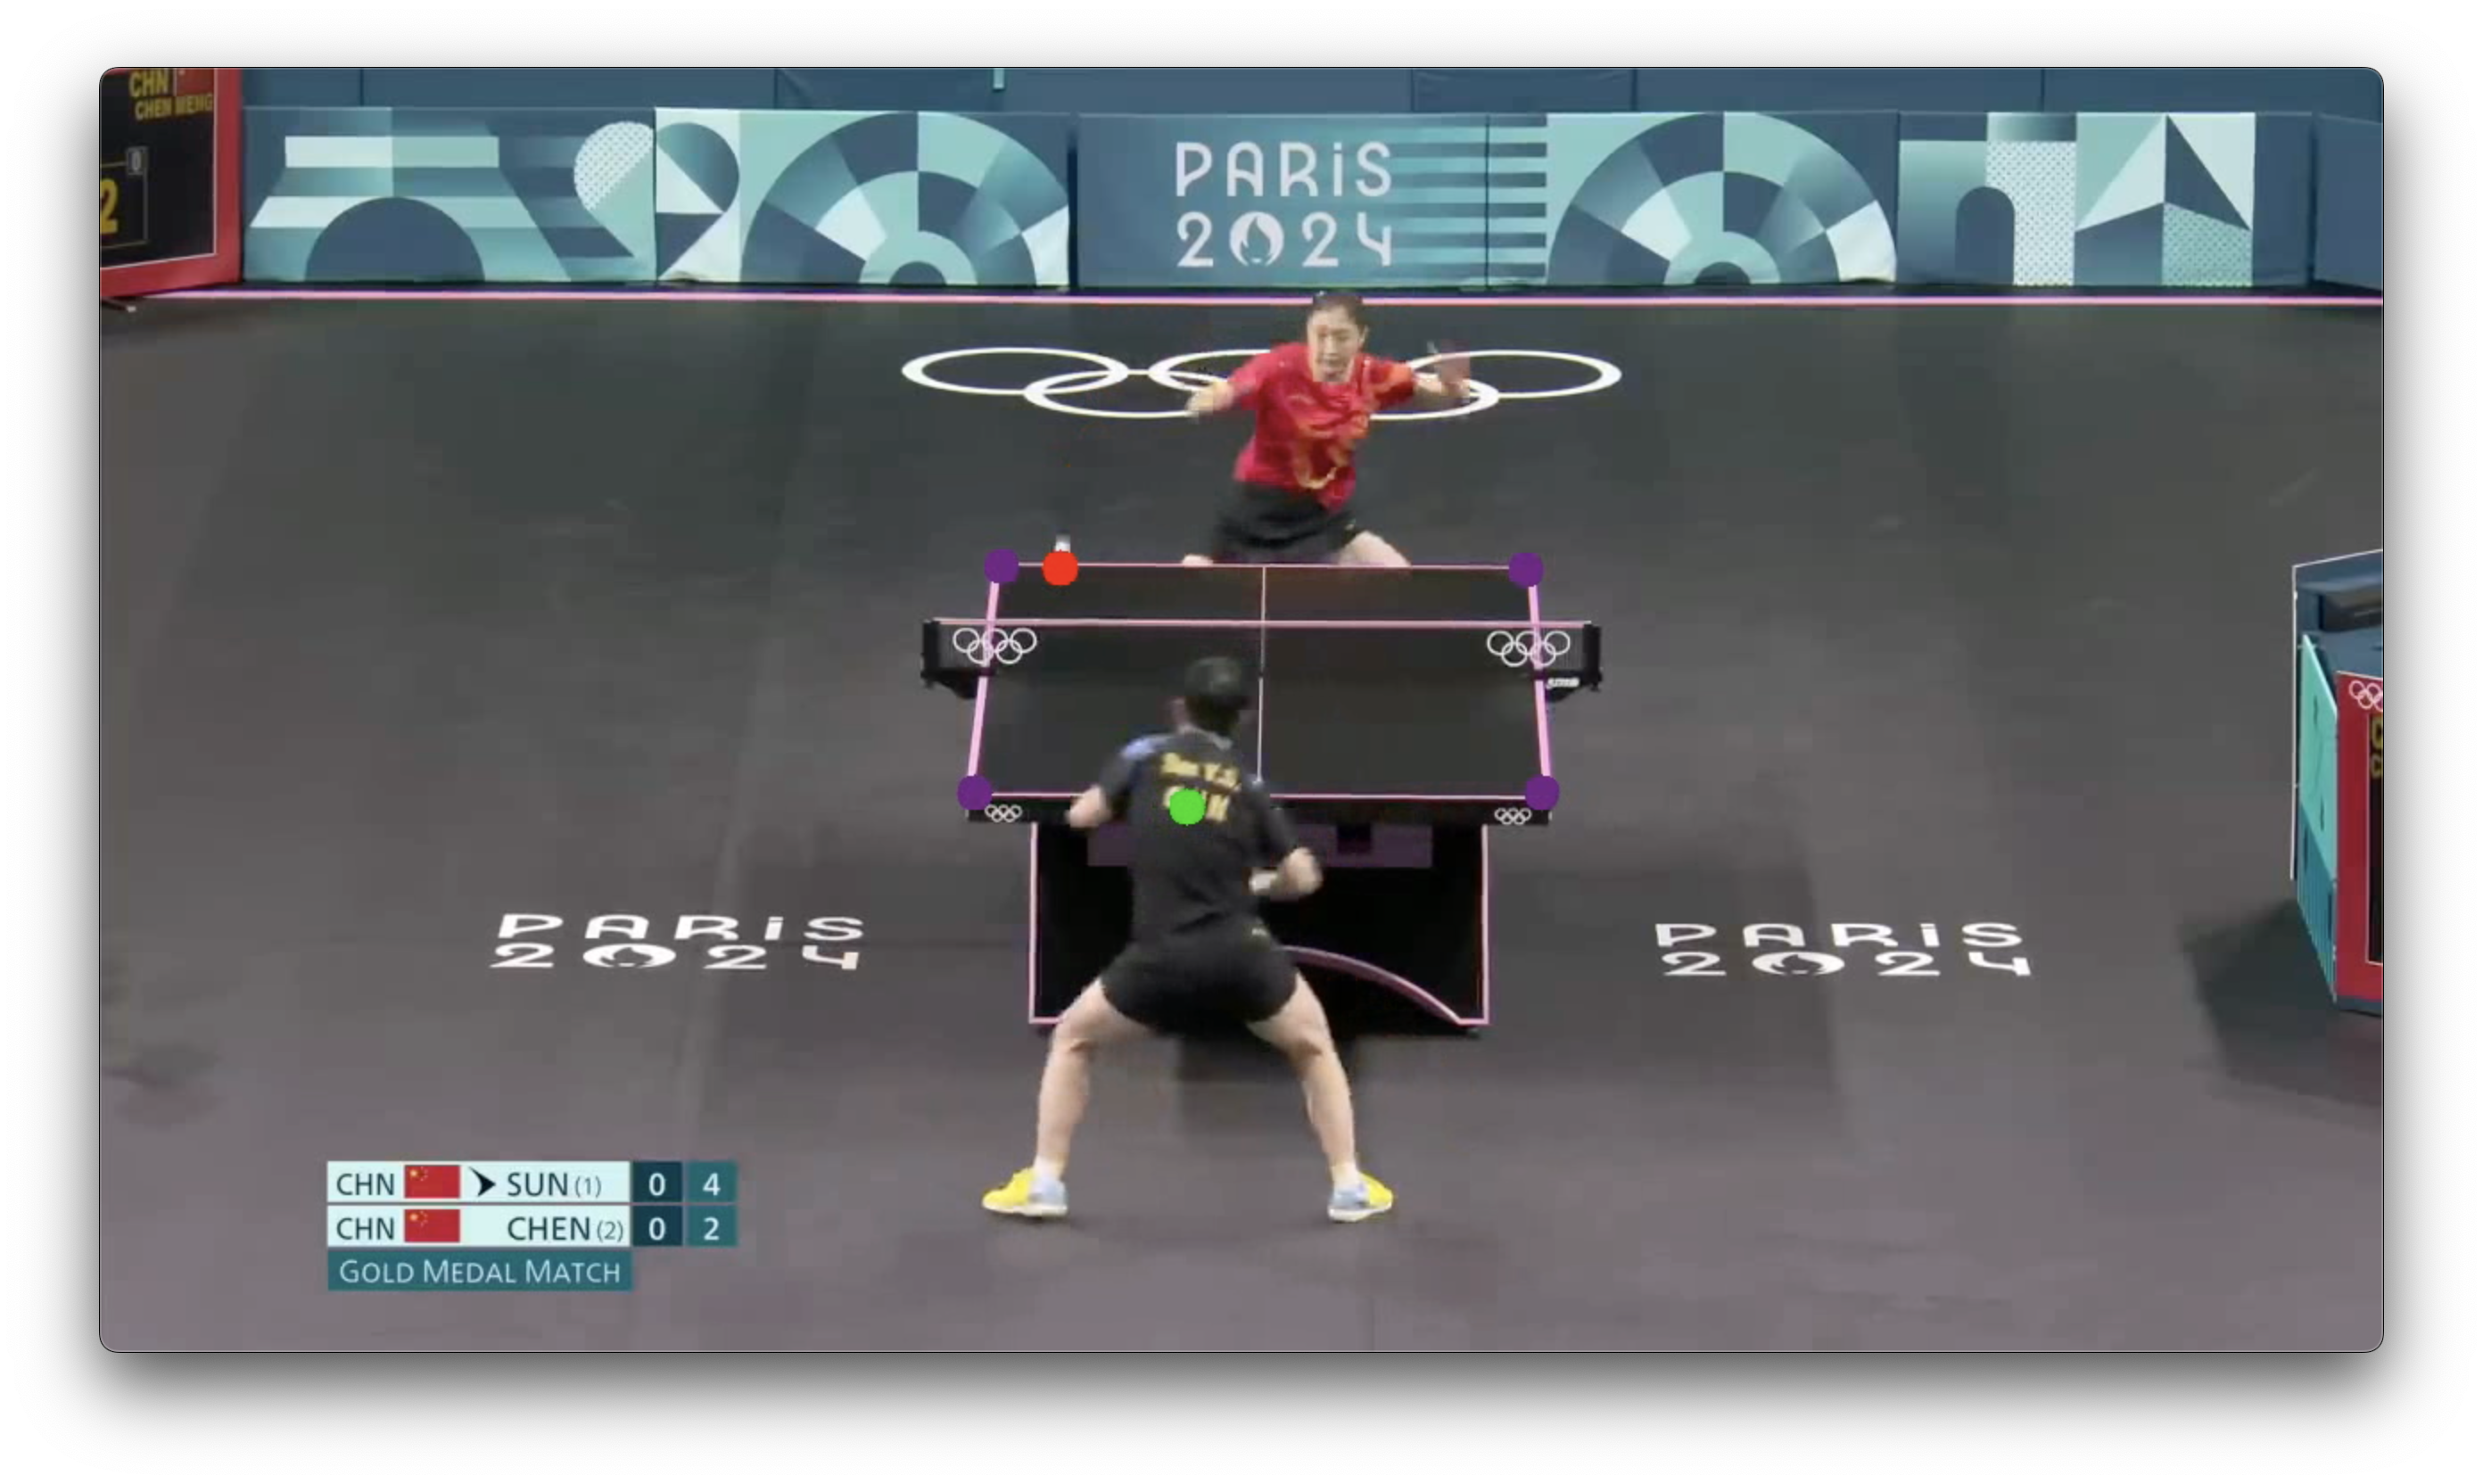}
\caption{Use the data collection pipeline for table tennis.}
\label{fig:table_tennis}
\end{figure}
